# Supplementary material for: Understanding Best Subset Selection: A Tale of Two C(omplex)ities
Source: arXiv:2301.06259 source file (2025-04-11)
Supplement: Supplementary file 1 [file fixed_feature_model_example.tex]

\subsection{Illustrative examples}
In this section, we will demonstrate the interplay between the two complexities and the identifiability margin through some easy examples.
We recall the linear model \eqref{eq: base model}. In this example, we will assume that the true support is $\cS = \{1\}$. For the design matrix $X$ we assume that the columns of $X$ are centered and normalized such that 
\[
\frac{\norm{X_j}_2}{\sqrt{n}} = 1, \quad \text{for all $j \in [p]$}. 
\]
\subsubsection{Block correlation}
In this section we consider the cross-correlation between the columns in the following way:

\[
  \frac{X_j^\top X_k}{n} = 
  \begin{cases}
    c & \text{for } j=1, k \neq 1 \\
    r & \text{for } j,k>1, j \neq k 
  \end{cases},
\]
where $0\leq c\leq r$. Thus we have the empirical covariance matrix to be 
\[
\widehat{\Sigma} := \frac{X^\top X}{n} = \begin{pmatrix}
    1 & c \mathbf{1}_{(p-1)}^\top \\
    c \mathbf{1}_{(p-1)} & \bG\\
\end{pmatrix},
\]
where $\bG = (1-r) \bbI_{(p-1)} + r \mathbf{1}_{(p-1)} \mathbf{1}_{(p-1)}^\top$. In this case

\[
\widehat{\tau}(1) = \beta_{1}^2 \min_{j \neq 1} \left\{ \frac{\norm{X_{1}}_2^2}{n} - \frac{(X_{1}^\top X_{j}/n)^2}{\norm{X_{j}}^2/n} \right\}  = \beta_1^2 (1- c^2).
\]
Next, we will analyze the geometric quantities.
In this case, we have 
\[
\widehat{\gamma}_j = \frac{X_{1} - \frac{X_j^\top X_{1}}{\norm{X_j}^2}.X_{j}}{\sqrt{\norm{X_{1}}^2 - \frac{(X_{1}^\top X_{j})^2}{\norm{X_{j}}^2}}}.
\] 
%{
% \color{red}
% What is the behaviour of 
% \[
% \sfd_\cT = \max_{j,k \neq 1} \norm{\widehat{\gamma}_j - \widehat{\gamma}_k}_2 = ??
% \]
% }

Note that \begin{align*}
    \norm{\widehat{\gamma}_j - \widehat{\gamma}_k}_2^2 & = 2 (1 - \widehat{\gamma}_j^\top \widehat{\gamma}_k)
\end{align*}
and 
\begin{align*}
    \widehat{\gamma}_j^\top \widehat{\gamma}_k &= \dfrac{\norm{X_{1}}^2/n - \frac{
    (X_j^\top X_{1}/n)^2 }{\norm{X_j}^2/n} - \frac{
    (X_k^\top X_{1}/n)^2 }{\norm{X_k}^2/n} +\frac{
    (X_j^\top X_{1}/n) (X_k^\top X_{1}/n) (X_j^\top X_{k}/n)}{(\norm{X_j}^2/n) (\norm{X_k}^2/n)}}{\sqrt{\norm{X_{1}}^2/n - \frac{(X_{1}^\top X_{j}/n)^2}{\norm{X_{j}}^2/n}} \sqrt{\norm{X_{1}}^2/n - \frac{(X_{1}^\top X_{k}/n)^2}{\norm{X_{k}}^2/n}}} = \frac{1 - 2c^2 + c^2 r}{1- c^2}.
\end{align*}
Hence, we have 
\[
 \norm{\widehat{\gamma}_j - \widehat{\gamma}_k}_2^2  = \frac{2 c^2(1-r)}{1-c^2}, \quad \text{for all $j,k\neq 1$}.
\]
If $p>4e$, then it follows that 
\begin{equation}
\label{eq: example_linear_space_complexity}
\frac{1}{8}\frac{c^2(1-r)}{1-c^2} \leq \ccEstar_{\cT_\emptyset}^2 \leq \ccE_{\cT_\emptyset}^2 \leq \frac{2 c^2(1-r)}{1-c^2}.
\end{equation}
For $j, k \neq 1$, let $\theta_{j,k}$ denote the
angle between $X_j$ and $X_k$. By standard algebra it follows that
\[
\norm{P_j- P_k}_{\op} = \sin(\theta_{j,k}) = \sqrt{1 - \cos^2(\theta_{j,k})} =  \sqrt{1 - \left( \frac{X_j^\top X_k}{\norm{X_j} \norm{X_k}}\right)^2} = \sqrt{1- r^2}.
\]
Hence, by similar argument, it follows that
\begin{equation}
\label{eq: example_projection_space_complexity}
\frac{1}{16}(1-r^2) \leq \ccEstar_{\cG_\emptyset}^2 \leq \ccE_{\cG_\emptyset}^2 \leq (1-r^2).
\end{equation}

\paragraph{Orthogonal design: }
In this case $c = r= 0$. In this case \eqref{eq: example_projection_space_complexity} suggest that $\ccE_{\cG_\emptyset}^2  \geq 1/16$. On the other hand \eqref{eq: example_linear_space_complexity} suggests that $\ccE^2_{\cT_\emptyset} = 0$. Thus, the complexity of spurious projections is dominant in this case. Also, in this case $\widehat{\tau}(1) = \beta_1^2$.

\paragraph{Orthogonal block design:} 
In this case, we set $c=0$ and we vary $r$ in $(0,1)$. Note that \eqref{eq: example_linear_space_complexity} tells that $\ccE_{\cT_\emptyset}^2 
 = 0$. On the other hand \eqref{eq: example_projection_space_complexity} suggests that $\ccE_{\cG_\emptyset}^2$ has a decreasing trend with $r \in (0,1)$. Noting the fact that $\widehat{\tau}(1) = \beta_1^2$, we can conclude that for high values of $r$ the sufficient condition in Theorem \ref{thm: sufficiency of BSS} becomes less stringent.

 \paragraph{Equicorrelated design:}
 Here we set $c = r $. Let $r_0, r_1$ be the solutions to the equations
 \[
 \frac{2 r^2}{1+r} - \frac{1}{16}(1-r^2)=0, \quad \text{and} \quad \frac{1}{8} \frac{r^2}{1+r} - (1-r^2) = 0
 \]
 respectively.
 Using \eqref{eq: example_linear_space_complexity} and \eqref{eq: example_projection_space_complexity} it follows that for $0\leq r <r_0$ the complexity of spurious projection operators is dominating, i.e.,
 \[
 \ccE_{\cG_{\emptyset}}^2 > \ccE_{\cT_\emptyset}^2.
 \]
 In contrast, for $r_1<r<1$ we have the complexity of the residualized signals to be dominating, i.e.,
 \[
 \ccE_{\cT_{\emptyset}}^2 > \ccE_{\cG_\emptyset}^2.
 \]
 It turns out that $r_1 >0.95$. Thus, for $r> r_1$ the identifiability margin $\widehat{\tau}(1) = \beta_1^2 (1-r^2)$ is very small. Hence, for model consistency, we need high value for $\beta_1^2$.

 \subsubsection{Auto-correlation}
 We set the cross-correlation between the columns to be 
 \[
 \frac{X_i^\top X_j}{n} = \rho^{\abs{i-j}}, \quad \text{for all $i \neq j$},
 \]
 where $\rho \in (0,1)$.
In this case

\[
\widehat{\tau}(1) = \beta_{1}^2 \min_{j \neq 1} \left\{ \frac{\norm{X_{1}}_2^2}{n} - \frac{(X_{1}^\top X_{j}/n)^2}{\norm{X_{j}}^2/n} \right\}  = \beta_1^2 (1- \rho^2).
\]
Next, for $1<k<j$ we have
\begin{align*}
    \widehat{\gamma}_j^\top \widehat{\gamma}_k &= \dfrac{\norm{X_{1}}^2/n - \frac{
    (X_j^\top X_{1}/n)^2 }{\norm{X_j}^2/n} - \frac{
    (X_k^\top X_{1}/n)^2 }{\norm{X_k}^2/n} +\frac{
    (X_j^\top X_{1}/n) (X_k^\top X_{1}/n) (X_j^\top X_{k}/n)}{(\norm{X_j}^2/n) (\norm{X_k}^2/n)}}{\sqrt{\norm{X_{1}}^2/n - \frac{(X_{1}^\top X_{j}/n)^2}{\norm{X_{j}}^2/n}} \sqrt{\norm{X_{1}}^2/n - \frac{(X_{1}^\top X_{k}/n)^2}{\norm{X_{k}}^2/n}}} = \sqrt{\frac{1 - \rho^{2k-2}}{1- \rho^{2j -2}}}.
\end{align*}
Hence, we have 
\[
 \norm{\widehat{\gamma}_j - \widehat{\gamma}_k}_2^2  = 2 \left(1 - \sqrt{\frac{1 - \rho^{2k-2}}{1- \rho^{2j -2}}}\right), \quad \text{for all $1<k<j\leq p$}.
\]
Thus we have 
\[
\sfd_{\cT_\emptyset}^2 = 2 \left(1 - \sqrt{\frac{1 - \rho^{2p-4}}{1- \rho^{2p -2}}}\right), \sfD_{\cT_\emptyset}^2 = 2 \left(1 - \sqrt{\frac{1 - \rho^{2}}{1- \rho^{2p -2}}}\right)
\]
By a similar calculation, we can also show that 
\[
\sfd_{\cG_\emptyset}^2 = (1 - \rho^{2}), \sfD_{\cG_\emptyset}^2 = (1 - \rho^{2p - 4}).
\]
Combining the above two displays we get
\[
\frac{1}{8} \left(1 - \sqrt{\frac{1 - \rho^{2p-4}}{1- \rho^{2p -2}}}\right) \leq \ccEstar^2_{\cT_\emptyset} \leq \ccE^2_{\cT_\emptyset} \leq 2 \left(1 - \sqrt{\frac{1 - \rho^{2}}{1- \rho^{2p -2}}}\right),
\]
and 
\[
\frac{1}{16}(1-\rho^2)
\leq \ccEstar^2_{\cG_\emptyset} \leq \ccE^2_{\cG_\emptyset} \leq (1 - \rho^{2p-4}).
\]
Let $\rho_{0}(p)$ and $\rho_1(p)$ be the solutions of the equations
\[
2 \left(1 - \sqrt{\frac{1 - \rho^{2}}{1- \rho^{2p -2}}}\right) - \frac{1}{16}(1-\rho^2) = 0, \quad \text{and} \quad \frac{1}{8} \left(1 - \sqrt{\frac{1 - \rho^{2p-4}}{1- \rho^{2p -2}}}\right) - (1- \rho^{2p-4}) = 0
\]
respectively. If $0 \leq \rho<\rho_0(p) $ then $\ccE^2_{\cT_\emptyset} < \ccE^2_{\cG_\emptyset}$. On the other hand if $\rho_1(p) < \rho <1$, then $\ccE^2_{\cT_\emptyset} > \ccE^2_{\cG_\emptyset}$.
