# Supplementary material for: Understanding Best Subset Selection: A Tale of Two C(omplex)ities
Source: arXiv:2301.06259 source file (2025-04-11)
Supplement: Supplementary file 2 [file initial_complexity_math.tex]

Recall that $\ccA_{s,k}:= \{\cD \subseteq \ccA_s : \abs{\cS\setminus \cD} = k\}$ and
\begin{equation}
\label{eq: Schur comp}
    \Delta(\cD) =  \widehat{\Sigma}_{ \cS \setminus \cD, \cS \setminus \cD} -  \widehat{\Sigma}_{ \cS \setminus \cD, \cD}\widehat{\Sigma}_{\cD, \cD}^{-1} \widehat{\Sigma}_{\cD, \cS \setminus \cD}
\end{equation}
Note that for a  constant $\eta>0$ and $\cD \in \ccA_{s,k}$ we have the following:
\begin{equation}
\label{eq: RSS diff}
    \begin{aligned}
    & n^{-1} (R_\cD - R_\cS) = n^{-1}\{ Y^\top (\bbI_n - P_\cD ) Y - Y^\top (\bbI_n - P_\cS) Y\}\\
    &= n^{-1} \left\{ (X_{\cS \setminus \cD} \beta_{\cS \setminus \cD} + E)^\top (\bbI_n - P_{\cD}) (X_{\cS \setminus \cD} \beta_{\cS \setminus \cD} + E) -  E^\top (\bbI_n - P_\cS) E \right\}\\
    & = \eta \beta_{\cD\setminus \cS}^\top \Delta(\cD) \beta_{\cS\setminus \cD} + 2^{-1}(1-\eta)  \beta_{\cS\setminus \cD}^\top \Delta(\cD) \beta_{\cS\setminus \cD} - 2 \left\{n^{-1} (\bbI_n - P_{\cD})X_{\cS\setminus \cD}\beta_{\cS\setminus \cD}\right\}^\top (-E)\\
    &\quad  + 2^{-1}(1-\eta)  \beta_{\cS\setminus \cD}^\top \Delta(\cD) \beta_{\cS\setminus \cD} - n^{-1} E^\top(P_\cD - P_\cS) E.
    \end{aligned}
\end{equation}
Also, let $\widetilde{E}:= (-E)$.
Now, note that BSS chooses the correct model if 
$$
\min_{\cD \in \ccA_s} n^{-1}(R_\cD - R_\cS) > 0.
$$
Hence, by union bound we have the following:

\begin{equation}
\label{eq: error prob BSS}
 \pr (\widehat{\cS}_{\rm best} \neq \cS) \leq \sum_{k =1}^s \pr \left( \min_{\cD \in \ccA_{s,k} } n^{-1} (R_\cD - R_\cS) <0\right). 
\end{equation}

Thus,  under the light of equation \eqref{eq: RSS diff} it is sufficient to show the following with high probability:

% \begin{equation}
%     \label{eq: quant 1}
%     \max_{\cD}\abs{ 2n^{-1} \left\{ (\bbI_n. - P_\cD)X_{\cS\setminus\cD}\beta_{\cS\setminus \cD}\right\}^\top E } < 2^{-1} (1-\eta) \beta_{\cS\setminus \cD}^\top \Delta(\cD) \beta_{\cS\setminus \cD}
% \end{equation}

% \begin{equation}
%     \label{eq: quant 2}
%     \max_{\cD}\abs{ n^{-1} \left\{ E^\top (\bbI_n - P_\cD) E \right\}} < 2^{-1} (1-\eta) \beta_{\cS\setminus \cD}^\top \Delta(\cD) \beta_{\cS\setminus \cD}
% \end{equation}

\begin{equation}
\label{eq: quant 1}
\max_{\cD \in \ccA_{s,k}} \widehat{\gamma}_\cD^\top \widetilde{E} < \frac{(1-\eta)n^{1/2}}{4} \min_{\cD\in \ccA_{s,k}} \norm{\gamma_\cD}_2,
\end{equation}

\begin{equation}
    \label{eq: quant 2}
    \max_{\cD\in \ccA_{s,k}} n^{-1} \left\{ E^\top (P_\cD - P_\cS) E \right\} < \frac{1 - \eta}{2} \min_{\cD\in \ccA_{s,k}}\norm{\gamma_\cD}_2^2,
\end{equation}
for every $k \in [s]$.
We will analyze the above events separately. We recall the two important spaces below:
\[
\cT_k:= \{ \widehat{\gamma}_\cD  : \cD \in \ccA_{s,k}  \},
\]

\[
\cG_k := \{ P_\cD  : \cD \in \ccA_{s,k} \}.
\]

\textbf{Linear term:} We begin with analyzing the supremum process in Equation \eqref{eq: quant 1}. First note the following:
\[
\max_{\cD\in \ccA_{s,k}} \widehat{\gamma}_{\cD}^\top \widetilde{E} = \max_{\cD\in \ccA_{s,k}} (\widehat{\gamma}_{\cD} - \widehat{\gamma}_{\cD_{0,k}})^\top \widetilde{E} + \widehat{\gamma}_{\cD_{0,k}}^\top \widetilde{E},
\]
where $\cD_{0,k} \in \ccA_{s,k} $ is a fixed subset such that $\norm{P_{\cD_{0,k}} - P_\cS}_{\op} = \sfd_{\cG_k}^\circ$.
Let $f_\cD : = (\widehat{\gamma}_{\cD} - \widehat{\gamma}_{\cD_{0,k}})^\top \widetilde{E} $ and $\norm{f} := \max_{\cD\in \ccA_{s,k}} f_\cD$.
By Borell-TIS inequality \citep[Theorem 2.1.1]{adler2007random}, we have 
\begin{equation}
\label{eq: borell-TIS}
\pr \left\{ \norm{f} - \bbE(\norm{f}) \geq \sigma u \right\} \leq \exp \left(- \frac{u^2}{2 \sfD^2_{\cT_k}}\right),
\end{equation}
for all $u>0$. Also, by Theorem 1 of Section 14 in \cite{lifshits1995gaussian} and using the fact that $\abs{\cT_k} = \binom{p-s}{k} \binom{s}{k}\leq (e p)^{2k}$, we have
\[
\bbE(\norm{f}) \leq 4\sqrt{2} \sigma \int_{0}^\infty \sqrt{\log \cN(\varepsilon, \cT_k, \norm{\cdot}_2)} \; \d\varepsilon \leq 8  \sfD_{\cT_k} \sigma \sqrt{k \log(ep)}.
\]
Setting $u = 2\sfD_{\cT_k}\sqrt{ k  \log(ep)}$ in Equation \eqref{eq: borell-TIS} we get 
\begin{equation}
\label{eq: linear deviation}
 \pr (\norm{f} \geq 10 \sfD_{\cT_k} \sigma \sqrt{ k \log(ep)}) \leq (ep)^{-2k}.
\end{equation}

Finally note that $\widehat{\gamma}_{\cD_{0,k}}^\top \widetilde{E} \sim N(0,1)$. Hence, $\pr(\widehat{\gamma}_{\cD_0}^\top \widetilde{E} \geq c_\cT \sigma \sqrt{  k \log(ep)}) \leq (ep)^{- c_\cT^2 k/2}$, where $c_\cT>0$ is an arbitrary constant. Thus, for $s\geq 1$ we have

\begin{equation}
\label{eq: linear deviation 2}
    \pr \left\{\max_{\cD \in \ccA_{s,k}} \widehat{\gamma}_{\cD}^\top \widetilde{E} \geq (10 \sfD_{\cT_k} + c_\cT) \sigma \sqrt{k \log(ep) }  \right\} \leq (ep)^{-2k} + (ep)^{-c_\cT^2 k/2}.
\end{equation}
% If $\sfd^2_\cT \log(p) \to \infty$, then  we can set $c_p = \sfd^2_\cT$ to get 
% \begin{equation}
% \label{eq: linear deviation 3}
%     \pr \left\{\max_{\cD \neq \cS} \widehat{\gamma}_{\cD}^\top \widetilde{E} \geq 6\sqrt{2}\sfd_\cT \sqrt{s \log(ep) } \right\} \leq (ep)^{-1} + (ep)^{-\sfd^2_\cT}.
% \end{equation}

\textbf{Quadratic term:}
Here we study the quadratic supremum process in Equation \eqref{eq: quant 2}. For a fixed constant $c_\cG>0$, by union bound we have,
\begin{equation}
    \label{eq: quad decomposition}
    \begin{aligned}
    &\pr \left\{ n^{-1}\max_{\cD \in \ccA_{s,k}} E^\top (P_\cD - P_\cS)E > \sigma^2 u + \sigma^2 c_\cG u_0\right\}\\
    & \leq \pr \left\{ n^{-1} E^\top (P_{\cD_{0,k}} - P_\cS)E > \sigma^2 u_0 c_\cG \right\} + \sum_{\cD \in \ccA_{s,k}} \pr \left\{ n^{-1} E^\top (P_\cD - P_{\cD_{0,k}})E > \sigma^2 u \right\}.
    \end{aligned}
\end{equation}

Now we will use Theorem 1.1 of \cite{rudelson2013hanson}. In particular, working out the explicit constants in the proof of the theorem we get,
\[
 \pr \left\{ n^{-1} E^\top (P_\cD - P_{\cD_{0,k}})E > \sigma^2 u \right\} \leq 2 \exp \left\{-  \min \left( \frac{n^2 u^2}{256 \norm{P_\cD - P_{\cD_{0,k}}}^2_F}, \frac{n u}{16\sqrt{2} \norm{P_\cD - P_{\cD_{0,k}}}_{\op}}\right) \right\}, \; \forall u>0.
\]
% Hence by replacing $u$ by $u/2$ we have
% \[
%  \pr \left\{ n^{-1} E^\top (P_\cD - P_{\cD_{0,k}
%  })E > \frac{\sigma^2 u}{2} \right\} \leq 2 \exp \left\{-  \min \left( \frac{n^2 u^2}{1024 \norm{P_\cD - P_{\cD_{0,k}}}^2_F}, \frac{n u}{32\sqrt{2} \norm{P_\cD - P_{\cD_0}}_{\op}}\right) \right\}.
% \]
Also note that for $\cD \in \ccA_{s,k}$
$$
\norm{P_\cD - P_{\cD_{0,k}}}_F^2 \leq \rank(P_\cD - P_{\cD_{0,k}}) \norm{P_\cD - P_{\cD_{0,k}}}_{\op}^2 \leq 4k \sfD^2_{\cG_k}.
$$
Thus,  we have
\begin{equation}
    \label{eq: quad deviation}
    \begin{aligned}
    %&\pr \left\{ n^{-1} E^\top (P_\cD - P_{\cD_{0,k}})E > \sigma^2 u(1 - c_\cG) \right\}\\
    & \leq \pr \left\{ n^{-1} E^\top (P_\cD - P_{\cD_{0,k}})E >  \sigma^2 u \right\}\\
    &\leq 2 \exp \left\{-  \min \left( \frac{n^2 u^2}{1024 k \sfD^2_{\cG_k}}, \frac{n u}{16\sqrt{2} \sfD_{\cG_k}}\right)  \right\}.
    \end{aligned}
\end{equation}
Setting $u = 4 \times \{16\sqrt{2} \sfD_{\cG_k} k \log (ep)/n\}$ we get 
\begin{equation}
    \label{eq: quad deviation 2}
     \pr \left\{ n^{-1} E^\top (P_\cD - P_{\cD_{0,k}})E > \frac{64 \sqrt{2} \sfD_{\cG_k} \sigma^2 k \log(ep)}{n} (1 - c_\cG) \right\} \leq 2 \exp \left\{-  4 k \log (ep)  \right\}.
\end{equation}
This shows that 
\begin{equation}
    \label{eq: quad deviation 3}
    \begin{aligned}
    &\pr \left\{ n^{-1}\max_{\cD \in \ccA_{s,k}} E^\top (P_\cD - P_{\cD_{0,k}})E > \frac{64 \sqrt{2} \sfD_{\cG_k} \sigma^2 k \log(ep)}{n}\right\}\\
    &\leq 2 \binom{p-s}{k} \binom{s}{k} \exp(- 4k \log(ep))\\
    &\leq 2(ep)^{-2k}.
    \end{aligned}
\end{equation}
By a similar argument, setting $u_0 = 4 \times \{16\sqrt{2} \sfd_{\cG_k}^\circ k \log (ep)/n\}$ we can show
\begin{equation}
    \label{eq: quad deviation 4}
    \begin{aligned}
    & \pr \left\{ n^{-1} E^\top (P_{\cD_{0,k}} - P_\cS)E > \frac{64 \sqrt{2}  c_\cG \sfd_{\cG_k}^\circ \sigma^2 k \log(ep)}{n}\right\}\\
    & \leq 2 \exp \left\{-  4c_\cG k \log(ep) \right\}\\
    & = 2 (ep)^{- 4 c_\cG k},
    \end{aligned}
\end{equation}
 Combining Equation \eqref{eq: quad deviation 3} and Equation \eqref{eq: quad deviation 4} yields

\begin{equation}
    \label{eq: quad deviation 5}
    \pr \left\{ n^{-1}\max_{\cD \in \ccA_{s,k}} E^\top (P_\cD - P_{\cS})E > 64 \sqrt{2} (\sfD_{\cG_k} + c_\cG \sfd^\circ_{\cG_k})\sigma^2\frac{ k \log(ep)}{n}\right\} \leq 2 (ep)^{-2k} + 2 (ep)^{-4 c_\cG k}.
\end{equation}
Setting $\eta = 0$ in Equation \eqref{eq: quant 1} and \eqref{eq: quant 2}, we have following requirements for vanishing error probability in Equation \eqref{eq: error prob BSS}:
\begin{itemize}
    \item 
    \[
     \min_{\cD \in \ccA_{s,k}}\frac{\norm{\gamma_\cD}_2}{\sqrt{k}} \geq 4(10 \sfD_{\cT_k} + c_\cT) \sigma \left\{ \frac{\log(ep)}{n}\right\}^{1/2}.
    \]
    
    \item $$\min_{\cD \in \ccA_{s,k}}\frac{\norm{\gamma_\cD}_2^2}{k} \geq 64 \sqrt{2} (\sfD_{\cG_k} + c_\cG \sfd^\circ_{\cG_k})\sigma^2 \left\{ \frac{\log(ep)}{n}\right\}.$$
\end{itemize}
Thus one sufficient condition for above condition to hold for all $k \in [s]$ is 
\begin{equation}
\label{eq: margin cond 1}
\widehat{\tau}(s) = \min_{\cD\neq \cS}\frac{\beta_{\cS\setminus \cD}^\top \Delta(\cD) \beta_{\cS\setminus \cD}}{\abs{\cS\setminus \cD}} \geq \max_{k \in [s]}\left\{16( 10 \sfD_{\cT_k} + c_\cT)^2, 64\sqrt{2} (\sfD_{\cG_k} + c_\cG \sfd^\circ_{\cG_k}) \right\} \sigma^2 \frac{\log(ep)}{n}.
\end{equation}
Thus, under \eqref{eq: margin cond 1}, Equation \eqref{eq: error prob BSS} yields

\begin{align*}
    \pr(\widehat{\cS}_{\rm best} \neq \cS) &\leq \sum_{k=1}^s (ep)^{-2k} + (ep)^{-c_\cT^2 k/2} + 2 (ep)^{-2k} + 2 (ep)^{-4 c_\cG k}\\
    & \leq 6 (ep)^{-2} + 2(ep)^{-c_\cT^2 /2} + 4 (ep)^{-4 c_\cG }.
\end{align*}
